# Supplementary material for: Design of High-Order Decoupled Multirate GARK Schemes
Source: arXiv:1804.07716 source file (2021-12-20)
Supplement: Supplementary file 1 [file MGARK_supplementary_material.tex]

%%%%%%%%%%%%%%%%%%%%%%%%%%%%%
\section{Two-partitioned trees of internally consistent methods up to order 4}
\label{sec:ptrees}
\bgroup

\begin{table}[hp]
\centering
\begin{tabular}{||c ||c ||}
    \hline\hline
    \begin{tikzpicture}[grow=up]\Tree [.\node[circle,draw,thick,fill=blue!50,opacity=0.5,label=right:$\tr{\b^{\{\s\}}}$](j){$\s$};  ]\end{tikzpicture} & \begin{tikzpicture}[grow=up]\Tree [.\node[circle,draw,thick,fill=red!50,opacity=0.5,label=right:$\tr{\b^{\{\f\}}}$](j){$\f$};  ]\end{tikzpicture}\\ \hline
%    $f^{\{\s\}}$ & $f^{\{\f\}}$\\ \hline
$t_{1}^{\langle 2,1 \rangle}$ & $t_{1}^{\langle 2,2 \rangle}$ \\ \hline
    $\tr{\b^{\{\s\}}}\mprod \one = 1$ & $\tr{\b^{\{\f\}}}\mprod \one = 1$ \\ \hline \hline
    \begin{tikzpicture}[grow=up]\Tree [.\node[circle,draw,thick,fill=blue!50,opacity=0.5,label=right:$\tr{\b^{\{\s\}}}$](j){$\s$}; [.\node[circle,draw,thick,fill=blue!50,opacity=0.5,label=right:$\c^{\{\s\}}$](k){$\s$};  ] ]\end{tikzpicture} & 
    \begin{tikzpicture}[grow=up]\Tree [.\node[circle,draw,thick,fill=red!50,opacity=0.5,label=right:$\tr{\b^{\{\f\}}}$](j){$\f$}; [.\node[circle,draw,thick,fill=red!50,opacity=0.5,label=right:$\c^{\{\f\}}$](k){$\f$};  ] ]\end{tikzpicture}\\ \hline
$t_{2}^{\langle 2,1 \rangle}$ & $t_{2}^{\langle 2,4 \rangle}$ \\ \hline
    $\tr{\b^{\{\s\}}} \mprod \c^{\{\s\}} = \frac{1}{2}$ & 
    $\tr{\b^{\{\f\}}} \mprod\c^{\{\f\}} = \frac{1}{2}$ \\ \hline \hline
\end{tabular}
\caption{N2T-trees up to order 2 for internally consistent methods.}
\label{tab:N2T-trees_1-2_intconsistent}
\end{table}

\begin{table}[hp]
\centering\begin{tabular}{||c ||c ||}
    \hline\hline
    \begin{tikzpicture}[grow=up]\Tree [.\node[circle,draw,thick,fill=blue!50,opacity=0.5,label=right:$\tr{\b^{\{\s\}}}$](j){$\s$}; [.\node[circle,draw,thick,fill=blue!50,opacity=0.5,label=right:$\c^{\{\s\}}$](l){$\s$};  ][.\node[circle,draw,thick,fill=blue!50,opacity=0.5,label=right:$\c^{\{\s\}}$](k){$\s$};  ] ]\end{tikzpicture} & \begin{tikzpicture}[grow=up]\Tree [.\node[circle,draw,thick,fill=red!50,opacity=0.5,label=right:$\tr{\b^{\{\f\}}}$](j){$\f$}; [.\node[circle,draw,thick,fill=red!50,opacity=0.5,label=right:$\c^{\{\f\}}$](l){$\f$};  ][.\node[circle,draw,thick,fill=red!50,opacity=0.5,label=right:$\c^{\{\f\}}$](k){$\f$};  ] ]\end{tikzpicture} \\ 
    \hline
$t_{3,1}^{\langle 2,1 \rangle}$ &  $t_{3,1}^{\langle 2,6 \rangle}$ \\ \hline
    $\tr{\b^{\{\s\}}} \mprod \c^{\{\s\} \times 2}= \frac{1}{3}$ & 
    $\tr{\b^{\{\f\}}} \mprod \c^{\{\f\} \times 2}= \frac{1}{3}$ \\ \hline \hline
    \begin{tikzpicture}[grow=up]\Tree [.\node[circle,draw,thick,fill=blue!50,opacity=0.5,label=right:$\tr{\b^{\{\s\}}}$](j){$\s$}; [.\node[circle,draw,thick,fill=blue!50,opacity=0.5,label=right:$ \A^{\{\s,\s\}}$](k){$\s$}; [.\node[circle,draw,thick,fill=blue!50,opacity=0.5,label=right:$ \c^{\{\s\}}$](l){$\s$};  ] ] ]\end{tikzpicture} & 
   \begin{tikzpicture}[grow=up]\Tree [.\node[circle,draw,thick,fill=blue!50,opacity=0.5,label=right:$\tr{\b^{\{\s\}}}$](j){$\s$}; [.\node[circle,draw,thick,fill=red!50,opacity=0.5,label=right:$ \A^{\{\s,\f\}}$](k){$\f$}; [.\node[circle,draw,thick,fill=red!50,opacity=0.5,label=right:$ \c^{\{\f\}}$](l){$\f$};  ] ] ]\end{tikzpicture} \\ \hline
$t_{3,2}^{\langle 2,1 \rangle}$ &  $t_{3,2}^{\langle 2,4 \rangle}$ \\ \hline
    $\tr{\b^{\{\s\}}} \mprod \A^{\{\s,\s\}} \mprod \c^{\{\s\}}= \frac{1}{6}$ &  
    $\tr{\b^{\{\s\}}} \mprod \A^{\{\s,\f\}} \mprod \c^{\{\f\}}= \frac{1}{6}$ \\ \hline \hline
    \begin{tikzpicture}[grow=up]\Tree [.\node[circle,draw,thick,fill=red!50,opacity=0.5,label=right:$\tr{\b^{\{\f\}}}$](j){$\f$}; [.\node[circle,draw,thick,fill=blue!50,opacity=0.5,label=right:$ \A^{\{\f,\s\}}$](k){$\s$}; [.\node[circle,draw,thick,fill=blue!50,opacity=0.5,label=right:$ \c^{\{\s\}}$](l){$\s$};  ] ] ]\end{tikzpicture} & 
 \begin{tikzpicture}[grow=up]\Tree [.\node[circle,draw,thick,fill=red!50,opacity=0.5,label=right:$\tr{\b^{\{\f\}}}$](j){$\f$}; [.\node[circle,draw,thick,fill=red!50,opacity=0.5,label=right:$\A^{\{\f,\f\}}$](k){$\f$}; [.\node[circle,draw,thick,fill=red!50,opacity=0.5,label=right:$ \c^{\{\f\}}$](l){$\f$};  ] ] ]\end{tikzpicture}   \\ \hline
$t_{3,2}^{\langle 2,5 \rangle}$ &  $t_{3,2}^{\langle 2,8 \rangle}$ \\ \hline
    $\tr{\b^{\{\f\}}} \mprod \A^{\{\f,\s\}} \mprod \c^{\{\s\}} = \frac{1}{6}$ &  
    $\tr{\b^{\{\f\}}} \mprod \A^{\{\f,\f\}} \mprod \c^{\{\f\}} = \frac{1}{6}$ \\ \hline \hline
    \end{tabular}
\caption{N2T-trees of order 3 for internally consistent methods.
}
\label{tab:N2T-trees_3_intconsistent}
\end{table}
\egroup
%%%%%%%%%%%%%%%%%%%%%%%
\section{Bi-colored trees for internally consistent schemes}

\bgroup

\begin{table}[hp]
\centering
\begin{tabular}{||c ||c ||}
\hline\hline
    \begin{tikzpicture}[grow=up]\Tree [.\node[circle,draw,thick,fill=blue!50,opacity=0.5,label=right:$\tr{\b^{\{\s\}}}$](j){$\s$}; [.\node[circle,draw,thick,fill=blue!50,opacity=0.5,label=right:$\c^{\{\s\}}$](m){$\s$};  ][.\node[circle,draw,thick,fill=blue!50,opacity=0.5,label=right:$\c^{\{\s\}}$](l){$\s$};  ][.\node[circle,draw,thick,fill=blue!50,opacity=0.5,label=right:$\c^{\{\s\}}$](k){$\s$};  ] ]\end{tikzpicture} & 
    \begin{tikzpicture}[grow=up]\Tree [.\node[circle,draw,thick,fill=red!50,opacity=0.5,label=right:$\tr{\b^{\{\f\}}}$](j){$\f$}; [.\node[circle,draw,thick,fill=red!50,opacity=0.5,label=right:$\c^{\{\f\}}$](m){$\f$};  ][.\node[circle,draw,thick,fill=red!50,opacity=0.5,label=right:$\c^{\{\f\}}$](l){$\f$};  ][.\node[circle,draw,thick,fill=red!50,opacity=0.5,label=right:$\c^{\{\f\}}$](k){$\f$};  ] ]\end{tikzpicture} \\ \hline
$t_{4,1}^{\langle 2,1 \rangle}$ &  $t_{4,1}^{\langle 2,8 \rangle}$ \\ \hline
    $\tr{\b^{\{\s\}}} \mprod \c^{\{\s\} \times 3} = \frac{1}{4}$ & 
    $\tr{\b^{\{\f\}}} \mprod \c^{\{\f\} \times 3} = \frac{1}{4}$ \\ \hline\hline
\end{tabular}
\caption{Internally consistent $N2T$-trees corresponding to $t_{4,1}$. In total there are 8 $N2T$-trees generated by $t_{4,1}$.}
\label{tab:N2t41_intconsist}
\end{table}

\begin{table}[hp] \centering
\begin{tabular}{||c ||c ||}
\hline\hline
    \begin{tikzpicture}[grow=up]\Tree [.\node[circle,draw,thick,fill=blue!50,opacity=0.5,label=right:$\tr{\b^{\{\s\}}}$](j){$\s$}; [.\node[circle,draw,thick,fill=blue!50,opacity=0.5,label=right:$\A^{\{\s,\s\}}$](l){$\s$}; [.\node[circle,draw,thick,fill=blue!50,opacity=0.5,label=right:$\c^{\{\s\}}$](m){$\s$};  ] ][.\node[circle,draw,thick,fill=blue!50,opacity=0.5,label=right:$\c^{\{\s\}}$](k){$\s$};  ] ]\end{tikzpicture} & 
  \begin{tikzpicture}[grow=up]\Tree [.\node[circle,draw,thick,fill=blue!50,opacity=0.5,label=right:$\tr{\b^{\{\s\}}}$](j){$\s$}; [.\node[circle,draw,thick,fill=red!50,opacity=0.5,label=right:$\A^{\{\s,\f\}}$](l){$\f$}; [.\node[circle,draw,thick,fill=red!50,opacity=0.5,label=right:$\c^{\{\f\}}$](m){$\f$};  ] ][.\node[circle,draw,thick,fill=blue!50,opacity=0.5,label=right:$\c^{\{\s\}}$](k){$\s$};  ] ]\end{tikzpicture}  \\ \hline
$t_{4,2}^{\langle 2,1 \rangle}$ &  $t_{4,2}^{\langle 2,4 \rangle}$ \\ \hline
    $\tr{\b^{\{\s\}}} \mprod\left( \c^{\{\s\}} \sprod \A^{\{\s,\s\}} \mprod \c^{\{\s\}}\right)= \frac{1}{8}$ & 
    $\tr{\b^{\{\s\}}} \mprod \left( \c^{\{\s\}}\sprod \A^{\{\s,\f\}} \mprod  \c^{\{\f\}} \right)= \frac{1}{8}$ \\ \hline\hline
    \begin{tikzpicture}[grow=up]\Tree [.\node[circle,draw,thick,fill=red!50,opacity=0.5,label=right:$\tr{\b^{\{\f\}}}$](j){$\f$}; [.\node[circle,draw,thick,fill=blue!50,opacity=0.5,label=right:$\A^{\{\f,\s\}}$](l){$\s$}; [.\node[circle,draw,thick,fill=blue!50,opacity=0.5,label=right:$\c^{\{\s\}}$](m){$\s$};  ] ][.\node[circle,draw,thick,fill=red!50,opacity=0.5,label=right:$\c^{\{\f\}}$](k){$\f$};  ] ]\end{tikzpicture} & 
   \begin{tikzpicture}[grow=up]\Tree [.\node[circle,draw,thick,fill=red!50,opacity=0.5,label=right:$\tr{\b^{\{\f\}}}$](j){$\f$}; [.\node[circle,draw,thick,fill=red!50,opacity=0.5,label=right:$\A^{\{\f,\f\}}$](l){$\f$}; [.\node[circle,draw,thick,fill=red!50,opacity=0.5,label=right:$\c^{\{\f\}}$](m){$\f$};  ] ][.\node[circle,draw,thick,fill=red!50,opacity=0.5,label=right:$\c^{\{\f\}}$](k){$\f$};  ] ]\end{tikzpicture} \\ \hline
$t_{4,2}^{\langle 2,13 \rangle}$ &  $t_{4,2}^{\langle 2,16 \rangle}$ \\ \hline
    $\tr{\b^{\{\f\}}} \mprod \left(\c^{\{\f\}} \sprod \A^{\{\f,\s\}} \c^{\{\s\}} \right)= \frac{1}{8}$ &
    $\tr{\b^{\{\f\}}} \mprod \left( \c^{\{\f\}} \sprod \A^{\{\f,\f\}} \mprod \c^{\{\f\}} \right)= \frac{1}{8}$ \\ \hline\hline
\end{tabular}
\caption{Internally consistent $N2T$-trees corresponding to $t_{4,2}$. In total there are 16 $N2T$-trees generated by $t_{4,2}$.}
\label{tab:N2t42_intconsist}
\end{table}

\begin{table}[hp] \centering
\begin{tabular}{||c ||c ||}
    \hline\hline
    \begin{tikzpicture}[grow=up]\Tree [.\node[circle,draw,thick,fill=blue!50,opacity=0.5,label=right:$\tr{\b^{\{\s\}}}$](j){$\s$}; [.\node[circle,draw,thick,fill=blue!50,opacity=0.5,label=right:$ \A^{\{\s,\s\}}$](k){$\s$}; [.\node[circle,draw,thick,fill=blue!50,opacity=0.5,label=right:$\c^{\{\s\}}$](m){$\s$};  ][.\node[circle,draw,thick,fill=blue!50,opacity=0.5,label=right:$\c^{\{\s\}}$](l){$\s$};  ] ] ]\end{tikzpicture} & 
    \begin{tikzpicture}[grow=up]\Tree [.\node[circle,draw,thick,fill=blue!50,opacity=0.5,label=right:$\tr{\b^{\{\s\}}}$](j){$\s$}; [.\node[circle,draw,thick,fill=red!50,opacity=0.5,label=right:$\A^{\{\s,\f\}}$](k){$\f$}; [.\node[circle,draw,thick,fill=red!50,opacity=0.5,label=right:$\c^{\{\f\}}$](m){$\f$};  ][.\node[circle,draw,thick,fill=red!50,opacity=0.5,label=right:$\c^{\{\f\}}$](l){$\f$};  ] ] ]\end{tikzpicture}\\ \hline
$t_{4,3}^{\langle 2,1 \rangle}$ &  $t_{4,3}^{\langle 2,6 \rangle}$ \\ \hline
    $\tr{\b^{\{\s\}}} \mprod \A^{\{\s,\s\}} \mprod \c^{\{\s\}\times 2} = \frac{1}{12}$ & 
    $\tr{\b^{\{\s\}}} \mprod \A^{\{\s,\f\}} \mprod \c^{\{\f\}\times 2} = \frac{1}{12}$ \\ \hline\hline
    \begin{tikzpicture}[grow=up]\Tree [.\node[circle,draw,thick,fill=red!50,opacity=0.5,label=right:$\tr{\b^{\{\f\}}}$](j){$\f$}; [.\node[circle,draw,thick,fill=blue!50,opacity=0.5,label=right:$\A^{\{\f,\s\}}$](k){$\s$}; [.\node[circle,draw,thick,fill=blue!50,opacity=0.5,label=right:$\c^{\{\s\}}$](m){$\s$};  ][.\node[circle,draw,thick,fill=blue!50,opacity=0.5,label=right:$\c^{\{\s\}}$](l){$\s$};  ] ] ]\end{tikzpicture} & 
    \begin{tikzpicture}[grow=up]\Tree [.\node[circle,draw,thick,fill=red!50,opacity=0.5,label=right:$\tr{\b^{\{\f\}}}$](j){$\f$}; [.\node[circle,draw,thick,fill=red!50,opacity=0.5,label=right:$\A^{\{\f,\f\}}$](k){$\f$}; [.\node[circle,draw,thick,fill=red!50,opacity=0.5,label=right:$\c^{\{\f\}}$](m){$\f$};  ][.\node[circle,draw,thick,fill=red!50,opacity=0.5,label=right:$\c^{\{\f\}}$](l){$\f$};  ] ] ]\end{tikzpicture}\\ \hline
 $t_{4,3}^{\langle 2,7 \rangle}$ &  $t_{4,3}^{\langle 2,12 \rangle}$\\ \hline
    $\tr{\b^{\{\f\}}} \mprod \A^{\{\f,\s\}} \mprod \c^{\{\s\}\times 2} = \frac{1}{12}$ & 
    $\tr{\b^{\{\f\}}} \mprod \A^{\{\f,\f\}} \mprod \c^{\{\f\}\times 2}  = \frac{1}{12}$ \\
\hline\hline
\end{tabular}
\caption{Internally consistent $N2T$-trees corresponding to $t_{4,3}$. In total there are 12 $N2T$-trees generated by $t_{4,3}$.}
\label{tab:N2t43_intconsist}
\end{table}

\begin{table}[hp] \centering
\begin{tabular}{||c ||c ||}
    \hline\hline
    \begin{tikzpicture}[grow=up]\Tree [.\node[circle,draw,thick,fill=blue!50,opacity=0.5,label=right:$\tr{\b^{\{\s\}}}$](j){$\s$}; [.\node[circle,draw,thick,fill=blue!50,opacity=0.5,label=right:$\A^{\{\s,\s\}}$](k){$\s$}; [.\node[circle,draw,thick,fill=blue!50,opacity=0.5,label=right:$\A^{\{\s,\s\}}$](l){$\s$}; [.\node[circle,draw,thick,fill=blue!50,opacity=0.5,label=right:$\c^{\{\s\}}$](m){$\s$};  ] ] ] ]\end{tikzpicture} & 
     \begin{tikzpicture}[grow=up]\Tree [.\node[circle,draw,thick,fill=blue!50,opacity=0.5,label=right:$\tr{\b^{\{\s\}}}$](j){$\s$}; [.\node[circle,draw,thick,fill=blue!50,opacity=0.5,label=right:$\A^{\{\s,\s\}}$](k){$\s$}; [.\node[circle,draw,thick,fill=red!50,opacity=0.5,label=right:$\A^{\{\s,\f\}}$](l){$\f$}; [.\node[circle,draw,thick,fill=red!50,opacity=0.5,label=right:$\c^{\{\f\}}$](m){$\f$};  ] ] ] ]\end{tikzpicture} \\ \hline
$t_{4,4}^{\langle 2,1 \rangle}$ &   $t_{4,4}^{\langle 2,4 \rangle}$ \\ \hline
    $\tr{\b^{\{\s\}}} \mprod \A^{\{\s,\s\}}\mprod \A^{\{\s,\s\}} \mprod \c^{\{\s\}} = \frac{1}{24}$ 
    & $\tr{\b^{\{\s\}}} \mprod \A^{\{\s,\s\}} \mprod \A^{\{\s,\f\}} \mprod \c^{\{\f\}} = \frac{1}{24}$ \\ \hline\hline
    \begin{tikzpicture}[grow=up]\Tree [.\node[circle,draw,thick,fill=blue!50,opacity=0.5,label=right:$\tr{\b^{\{\s\}}}$](j){$\s$}; [.\node[circle,draw,thick,fill=red!50,opacity=0.5,label=right:$\A^{\{\s,\f\}}$](k){$\f$}; [.\node[circle,draw,thick,fill=blue!50,opacity=0.5,label=right:$\A^{\{\f,\s\}}$](l){$\s$}; [.\node[circle,draw,thick,fill=blue!50,opacity=0.5,label=right:$\c^{\{\s\}}$](m){$\s$};  ] ] ] ]\end{tikzpicture} & 
    \begin{tikzpicture}[grow=up]\Tree [.\node[circle,draw,thick,fill=blue!50,opacity=0.5,label=right:$\tr{\b^{\{\s\}}}$](j){$\s$}; [.\node[circle,draw,thick,fill=red!50,opacity=0.5,label=right:$\A^{\{\s,\f\}}$](k){$\f$}; [.\node[circle,draw,thick,fill=red!50,opacity=0.5,label=right:$\A^{\{\f,\f\}}$](l){$\f$}; [.\node[circle,draw,thick,fill=red!50,opacity=0.5,label=right:$\c^{\{\f\}}$](m){$\f$};  ] ] ] ]\end{tikzpicture} \\ \hline    
$t_{4,4}^{\langle 2,5 \rangle}$ &   $t_{4,4}^{\langle 2,8 \rangle}$ \\ \hline
    $\tr{\b^{\{\s\}}} \mprod \A^{\{\s,\f\}} \mprod \A^{\{\f,\s\}} \mprod  \c^{\{\s\}} = \frac{1}{24}$ & 
    $\tr{\b^{\{\s\}}} \mprod \A^{\{\s,\f\}} \mprod \A^{\{\f,\f\}} \mprod  \c^{\{\f\}} = \frac{1}{24}$ \\     \hline\hline
        \begin{tikzpicture}[grow=up]\Tree [.\node[circle,draw,thick,fill=red!50,opacity=0.5,label=right:$\tr{\b^{\{\f\}}}$](j){$\f$}; [.\node[circle,draw,thick,fill=blue!50,opacity=0.5,label=right:$\A^{\{\f,\s\}}$](k){$\s$}; [.\node[circle,draw,thick,fill=blue!50,opacity=0.5,label=right:$\A^{\{\s,\s\}}$](l){$\s$}; [.\node[circle,draw,thick,fill=blue!50,opacity=0.5,label=right:$\c^{\{\s\}}$](m){$\s$};  ] ] ] ]\end{tikzpicture} & 
         \begin{tikzpicture}[grow=up]\Tree [.\node[circle,draw,thick,fill=red!50,opacity=0.5,label=right:$\tr{\b^{\{\f\}}}$](j){$\f$}; [.\node[circle,draw,thick,fill=blue!50,opacity=0.5,label=right:$\A^{\{\f,\s\}}$](k){$\s$}; [.\node[circle,draw,thick,fill=red!50,opacity=0.5,label=right:$\A^{\{\s,\f\}}$](l){$\f$}; [.\node[circle,draw,thick,fill=red!50,opacity=0.5,label=right:$\c^{\{\f\}}$](m){$\f$};  ] ] ] ]\end{tikzpicture} \\ \hline
$t_{4,4}^{\langle 2,9 \rangle}$ &  $t_{4,4}^{\langle 2,12 \rangle}$ \\ \hline
    $\tr{\b^{\{\f\}}} \mprod \A^{\{\f,\s\}} \mprod \A^{\{\s,\s\}} \mprod  \c^{\{\s\}} = \frac{1}{24}$ & 
    $\tr{\b^{\{\f\}}} \mprod \A^{\{\f,\s\}} \mprod \A^{\{\s,\f\}} \mprod  \c^{\{\f\}} = \frac{1}{24}$ \\ 
\hline\hline
    \begin{tikzpicture}[grow=up]\Tree [.\node[circle,draw,thick,fill=red!50,opacity=0.5,label=right:$\tr{\b^{\{\f\}}}$](j){$\f$}; [.\node[circle,draw,thick,fill=red!50,opacity=0.5,label=right:$\A^{\{\f,\f\}}$](k){$\f$}; [.\node[circle,draw,thick,fill=blue!50,opacity=0.5,label=right:$\A^{\{\f,\s\}}$](l){$\s$}; [.\node[circle,draw,thick,fill=blue!50,opacity=0.5,label=right:$\c^{\{\s\}}$](m){$\s$};  ] ] ] ]\end{tikzpicture} & 
   \begin{tikzpicture}[grow=up]\Tree [.\node[circle,draw,thick,fill=red!50,opacity=0.5,label=right:$\tr{\b^{\{\f\}}}$](j){$\f$}; [.\node[circle,draw,thick,fill=red!50,opacity=0.5,label=right:$\A^{\{\f,\f\}}$](k){$\f$}; [.\node[circle,draw,thick,fill=red!50,opacity=0.5,label=right:$\A^{\{\f,\f\}}$](l){$\f$}; [.\node[circle,draw,thick,fill=red!50,opacity=0.5,label=right:$\c^{\{\f\}}$](m){$\f$};  ] ] ] ]\end{tikzpicture} \\ \hline
$t_{4,4}^{\langle 2,13 \rangle}$ &  $t_{4,4}^{\langle 2,16 \rangle}$ \\ \hline
    $\tr{\b^{\{\f\}}} \mprod \A^{\{\f,\f\}} \mprod \A^{\{\f,\s\}} \mprod  \c^{\{\s\}} = \frac{1}{24}$ & 
    $\tr{\b^{\{\f\}}} \mprod \A^{\{\f,\f\}} \mprod \A^{\{\f,\f\}} \mprod  \c^{\{\f\}} = \frac{1}{24}$\\     \hline\hline
    \end{tabular}
\caption{Internally consistent $N2T$-trees corresponding to $t_{4,4}$. In total there are 16 $N2T$-trees generated by $t_{4,4}$.}
\label{tab:N2t44_intconsist}
\end{table}
\egroup
